# Supplementary material for: Unlocking Out-of-Distribution Generalization in Transformers via Recursive Latent Space Reasoning
Source: arXiv:2510.14095 source file (2025-10-15)
Supplement: Supplementary file 1 [file additional_operations.tex]

\section{Experiments with Multiple Operations}\label{sec:experiments_additional_operations}

The experiments presented in the main paper were focused on a task with a single operation---modular addition. The reason for this is that our end-to-end and chain-of-thought baselines failed to generalized out-of-distribution even for this simpler setting. In this section, we evaluate our proposed method on a more complex version of the task with multiple modular arithmetic operations. We find that our architectural mechanisms continue to enable robust out-of-distribution generalization.
