# Supplementary material for: Unlocking Out-of-Distribution Generalization in Transformers via Recursive Latent Space Reasoning
Source: arXiv:2510.14095 source file (2025-10-15)
Supplement: Supplementary file 2 [file our_method_full.tex]

\section{Reasoning in Latent Space with Algorithmic Supervision}\label{sec:our_method}

\subsection{Mechanisms for Effective OOD Generalization.} \label{subsec:mechanisms}

% paragraph explaining challenges faced by standard methods such as CoT

Effective OOD generalization on complex reasoning tasks hinges on a model's ability to learn and emulate an underlying scalable \textit{algorithm}. This requires the model to, implicitly or explicitly, execute an iterative procedure that adapts to input complexity. Designing \emph{inductive biases} to support the discovery of such scalable, compositional solutions is a central challenge in machine learning~\citep{baxter2000model,lake2018generalization,barrett2018measuring,goyal2022inductive}. Chain-of-thought (CoT) techniques attempt this by having the model generate textual token representations of computational steps. However, this restriction to a token-based, autoregressive format often yields brittle ``algorithms" that fail to generalize robustly, especially as longer CoT sequences are needed for more complex inputs. These well-documented length generalization issues~\citep{anilExploringLengthGeneralization2022,kazemnejadImpactPositionalEncoding2023,jelassi2023lengthgeneralizationarithmetictransformers,zhouWhatAlgorithmsCan2023,stechly2024chain,zhouTransformersCanAchieve2024} underscore CoT's limitations in effectively emulating truly scalable algorithmic procedures. This work, therefore, proposes alternative mechanisms to facilitate the learning of such iterative algorithms directly within a model's latent operations. Our proposal features recurrent Transformer  blocks, algorithmic supervision and discretization in latent space, and a self-correction scheme. 
Collectively, these mechanisms constitute an architecture enabling native latent-space reasoning, leading to effective OOD generalization. See \Cref{fig:architecture_diagram} for an illustration of our proposal.

% This section proposes and explores architectural mechanisms and training methodologies designed to promote robust and scalable solutions for out-of-distribution generalization. Collectively, these mechanisms constitute an architecture enabling native latent-space reasoning, featuring an input-adaptive recurrent structure, trained with algorithmic supervision.

% Robust out-of-distribution generalization requires learning a universal and scalable \textit{algorithm} for solving the underlying task. In particular, the model must implicitly or explicitly learn an iterative algorithmic procedure that naturally scales with input complexity. Designing inductive biases to support the discovery of such scalable, compositional solutions is a central challenge in machine learning~\citep{baxter2000model,lake2018generalization,barrett2018measuring,goyal2022inductive}. While chain-of-thought techniques attempt to achieve this by allowing the model to generate a token representation of a computational process, restricting the model to reasoning in this token-based linear format can result in brittle algorithms. These often fail to scale or generalize far beyond the training distribution, particularly as the required CoT length grows with input complexity. These length generalization issues represent a critical challenge, studied extensively in prior work~\citep{
% anilExploringLengthGeneralization2022,kazemnejadImpactPositionalEncoding2023,jelassi2023lengthgeneralizationarithmetictransformers,zhouWhatAlgorithmsCan2023,stechly2024chain,zhouTransformersCanAchieve2024}.

\begin{figure}
    \centering
    \resizebox{\linewidth}{!}{
        \input{figs/architecture_diagram_recurrent}
    }
    \caption{Overview of the proposed architecture for OOD generalization. It features a recurrent Transformer block, latent algorithmic supervision, and a discretization mechanism to anchor representations across iterations. Self-correction mechanism is omitted. }\label{fig:architecture_diagram}
    \vskip-12pt
\end{figure}

\begin{mechanism}\label{mech:recurrence}
    Recurrence \& Input-Adaptive Computation
\end{mechanism}

At a minimum, systematic generalization to more complex input instances requires an ability for the model to scale its computation time proportionate to the requirements of these novel input instance, scaling beyond the training regime. We propose doing this via a \textit{recurrent architecture}, which allows us to scale computation time by scaling the number of recurrent iterations. Compared to scaling computation by generating more tokens (as in CoT), recurrence introduces inductive biases favoring recursive solution structures, which are inherently more scalable. This approach also offers computational advantages by enabling parallel processing within each step---unlike the linear CoT format---and operating with smaller context windows, as the full computational trace is not materialized sequentially. Recurrence is a central idea in machine learning, and has been explored in the context of scaling computation time in several prior works~\citep{gravesAdaptiveComputationTime2017,dehghaniUniversalTransformers2019,fanLoopedTransformersLength2024,geipingScalingTestTimeCompute2025}.

\vspace{5pt}
\begin{implementation}
    We use a recurrent Transformer architecture. The recurrent module is an $L$-layer Transformer, where each layer consists of multi-head attention followed by a position-wise MLP. This module is applied recurrently to iteratively process the input. We scale the number of recurrent iterations $T$ with the complexity of the input, scaling it linearly with the depth of the underlying computation graph.
    Given an input sequence of tokens $X = (x_1, \ldots, x_n)$, we embed it to form a sequence of embedding vectors $E_1^{(0)}, \ldots, E_n^{(0)}$ and recurrently process it with the $\mathrm{RecurrentTransformerBlock}$
    \begin{equation}\label{eq:recurrent_block}
        \begin{aligned}
            (E_1^{(t+1)}, \ldots, E_n^{(t+1)}) &\gets \mathrm{RecurrentTransformerBlock}(E_1^{(t)}, \ldots, E_n^{(t)}), \ t = 1, 2, \ldots, T.
        \end{aligned}
    \end{equation}
    The output is linearly read out from the final embedding states $E_1^{(T)}, \ldots, E_n^{(T)}$.
\end{implementation}

\begin{mechanism}\label{mech:latent_alg_sup}
    Latent State Algorithmic Supervision
\end{mechanism}
To aid the model in discovering a systematic and scalable algorithm, we provide algorithmic supervision, similar to CoT supervision, to align its internal states with a reference algorithmic procedure. Crucially, however, rather than providing this supervision by having the model generate a sequence of tokens, we provide this supervision \textit{directly in its latent space across recurrent iterations}. In this task, the goal of the algorithmic supervision is to steer the model to an algorithm that computes the computation graph one layer at a time.

% emphasize algorithm more clearly
% use figure as example (e.g., for t = 2 in Figure, Depth(x_i) includes nodes blah blah...

\begin{implementation}
    We aim to align the model with an algorithm that processes the input computation graph by computing variable values for one additional layer of depth per recurrent iteration. We do this by providing supervision in the latent states at each recurrent iteration. In particular, rather than having the readout layer predict the values only in the final layer, we apply the same read-out layer at \textit{every} recurrent iteration and compute a loss for each iteration, but penalizing prediction errors only for nodes at a graph depth less than or equal to the current iteration number $t$. In particular, for an input sequence $X = (x_1, \ldots, x_n)$, we compute the latent states $E_i^{(t)}$ for each iteration according to~\eqref{eq:recurrent_block}, and define the loss at iteration $t$ as
    \begin{equation}
        \mathtt{ValuePredictionLoss}(\mathrm{iteration} = t) = \sum_{\substack{i \in [n] \\ \mathtt{Depth}(x_i) \leq t}} \ell\paren{W_{\mathtt{value}} \,E_i^{(t)}, \mathtt{Value}(x_i)}.
        % \Ind{\mathrm{Syntax}(x_i) = \mathtt{variable}, \mathrm{Depth}(x_i) \leq t}.
    \end{equation}
    where $W_{\mathtt{value}}$ is the learned linear read-out layer for the node values, $\mathtt{Depth}(x_i)$ is the depth of the variable $x_i$ in the input computation graph, $\mathtt{Value}(x_i)$ is its value, and $E_i^{(t)} \in \reals^{d_\mathrm{model}}$ is the vector embedding of $x_i$ at recurrent iteration $t$. Here, $\ell$ is the cross-entropy loss. $W_{\mathtt{value}}$ is learned concurrently with the rest of the model parameters.

    The overall value prediction loss used to train the models is the sum of the losses at each iteration
    \begin{equation}
        \mathtt{ValuePredictionLoss} = \sum_{t} \mathtt{ValuePredictionLoss}(\mathrm{iteration} = t).
    \end{equation}
\end{implementation}

\begin{mechanism}\label{mech:discrete_states}
    Anchoring Latent Representation via Discretization
\end{mechanism}

One challenge that arises in such recurrent models with an input-adaptive number of iterations is that their internal vector representations begin to deviate from the original representation space when they are applied for a much greater number of iterations than they are trained on (which is required to solve much larger and more complex problem instances). Eventually, this representational drift accumulates, causing embeddings to deviate sufficiently from the learned manifold such that model performance on these larger inputs degrades. To address this challenge, we introduce a discretization mechanism in between recurrent computational blocks to \textit{anchor} the representations to a shared space across computational depth. This implements a type of discrete latent bottleneck, a type of information bottleneck~\citep{tishby2015deeplearninginformationbottleneck}, that promotes systematic generalization and scalability across very large computational depths.
The use of discrete representations in neural models has been explored in different contexts in prior work~\citep{jangCategoricalReparameterizationGumbelSoftmax2017,oordNeuralDiscreteRepresentation2018,smolensky2024mechanismssymbolprocessingincontext}.

\begin{implementation}
    As depicted in~\Cref{fig:architecture_diagram}, this mechanism anchors the model's latent representations by passing them through a discrete bottleneck after each recurrent block iteration, mapping to a discrete space before re-embedding for the subsequent iteration.

    The discrete space has a factored structure with four components: syntax, variable, operation, and value. We train linear layers for each factor $W_{\mathtt{factor}} \in \reals^{d_{\mathrm{model} \times \aabs{\calV_{\mathtt{factor}}}}}$ that map the vector state at the end of each recurrent iteration to a discrete prediction for each factor. This combines with the latent state supervision described in~\Cref{mech:latent_alg_sup}.

    % Each token's discrete state evolves within this discrete space over the course of the model's recurrent iterations. More specifically, the syntax, variable, and operation components remain fixed, while the value components change as the model computes the values of more nodes throughout its execution. For example, in the input ``$\token{17} \token{\to} \token{x_{42}} \sep ...$'', we tokenize $\token{17}$ and $\token{x_42}$ as follows
    As an example, at the zero-th layer, the tokens $\token{20}$ and $\token{x_{7}}$ are mapped to the following initial discrete states.
    \begin{center}
    \begin{tabular}{ccrccccl}
         &  & & \texttt{syntax} & \texttt{variable} & \texttt{operation} & \texttt{value} & \\[8pt]
        $\token{20}$ & $\to$ & $[$ & $\mathtt{value}$ & $\mathtt{N/A}$ & $\mathtt{N/A}$ & $20$ & $]$\\
         $\token{x_{7}}$& $\to$ & $[$ & $\mathtt{variable}$ & $x_{7}$ & $\mathtt{N/A}$ & $\mathtt{empty}$ & $]$\\
    \end{tabular}
    \end{center}
    We train a separate embedding layer for each factor and map the input to vector embeddings by embedding each component of the discrete state and adding the embeddings. The model iteratively updates the state of each node by computing node values one layer at a time, as described in~\Cref{mech:latent_alg_sup}.

    The recurrent iterations in~\Cref{eq:recurrent_block} are modified to incorporate the discretization mechanism as follows:
    \begin{equation}
    \begin{aligned}
        (E_1^{(t)}, \ldots, E_n^{(t)}) &\gets \mathrm{RecurrentTransformerBlock}(x_1^{(t)}, \ldots, x_n^{(t)})\\
        z_{i, \mathtt{factor}}^{(t+1)} &\gets \argmax \sset{W_{\mathtt{factor}} \, E_i^{(t)} } \quad \hphantom{~} \texttt{// discretize}\\%\quad \mathtt{factor} \in \sset{ \mathtt{syntax}, \mathtt{variable}, \mathtt{operation}, \mathtt{value}} \\
        x_{i, \mathtt{factor}}^{(t+1)} &\gets \mathrm{FactorEmbed}(z_{i, \mathtt{factor}}^{(t+1)}) \quad \texttt{// re-embed}\\%\quad \mathtt{factor} \in \sset{ \mathtt{syntax}, \mathtt{variable}, \mathtt{operation}, \mathtt{value}} \\
        x_i^{(t+1)} &\gets x_{i, \mathtt{syntax}}^{(t+1)} + x_{i, \mathtt{variable}}^{(t+1)} + x_{i, \mathtt{operation}}^{(t+1)} + x_{i, \mathtt{value}}^{(t+1)}
    \end{aligned}
    \end{equation}

    When using this discretization mechanism and the algorithmic supervision of~\Cref{mech:latent_alg_sup}, we train with teacher-forcing across recurrent depth.
\end{implementation}

\begin{mechanism}\label{mech:err_correct}
    Learning to Self-Correct
\end{mechanism}

In a reasoning task, each reasoning step depends crucially on the prior steps in the reasoning path. If a mistake is made at any stage, all subsequent computation is affected, and the error is often fatal. As the size of the problem and the number of computational steps scale, the likelihood of an error occurring at \textit{some point} in the reasoning process becomes large, limiting the ability to generalize indefinitely to more complex problems. To address this challenge, a reasoning model must be able to detect and correct errors as they occur in order to recover when a mistake is made in its previous computation.

\begin{implementation}
    We train the model to detect and correct errors by randomly corrupting the model's latent state. That is, at each iteration, with some small probability, we corrupt a random selection of the value components of the models' discrete states. To achieve good loss, the model must learn to detect when a previously-computed value is incorrect and correct it before proceeding.
\end{implementation}

\begin{table}
    \caption{\textit{Guide to Implementation of Proposed Mechanisms in Baselines.} The leftmost column shows the method names of the different baselines and ablations we consider, matching figure legends. $\checkmark$ indicates that a method implements the given mechanism, $\crossmark$ indicate that the mechanism is not implemented, and $\crosscheck$ indicate that it is partially implemented.}\label{tab:method_guide}
    \centering
    \resizebox{\textwidth}{!}{
    \begin{tabular}{ccccc}
        \toprule
        \textit{Method} / \textit{Mechanism} & \Cref{mech:recurrence} & \Cref{mech:latent_alg_sup} &  \Cref{mech:discrete_states}  & \Cref{mech:err_correct}\\\midrule
        \methodcolorhighlight{feedforwardcolor}{Feedforward End-to-End} & \crossmark & \crossmark & \crossmark & \crossmark\\
        \methodcolorhighlight{recurrentcolor}{Recurrent End-to-End} & \crosscheck & \crossmark & \crossmark & \crossmark\\
        % \methodcolorhighlight{feedforwardcolor}{End-to-End} & \crossmark & \crossmark & \crossmark & \crossmark\\
        \methodcolorhighlight{cotsupervisioncolor}{Chain-of-Thought} & \crosscheck & \crosscheck & \crossmark & \crossmark \\
        \methodcolorhighlight{continuoussupervisioncolor}{Continuous Latent Space Supervision} & \checkmark & \checkmark & \crossmark & \crossmark\\
        \methodcolorhighlight{discretesupervisioncolor}{Discrete Latent Space Supervision} & \checkmark & \checkmark & \checkmark & \crossmark\\
         \methodcolorhighlight{discretesupervisionrecorrectioncolor}{Discrete Latent Space Supervision $\circlearrowleft$}& \checkmark & \checkmark & \checkmark & \checkmark\\\bottomrule
    \end{tabular}
    }
\end{table}

\begin{figure}[h]
    \begin{minipage}{0.52\textwidth}
        \centering
        \includegraphics[width=\linewidth]{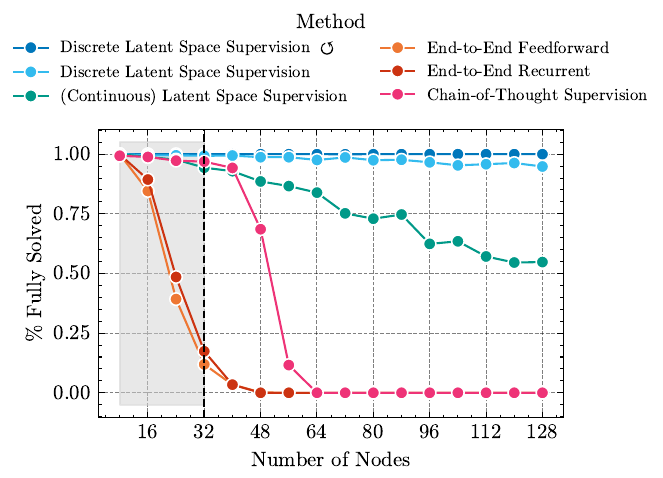}
        \captionof{figure}{Out-of-Distribution generalization performance of different methods on the mathematical reasoning task.}
        \label{fig:method_ood_comparison}
    \end{minipage}%
    \hfill
    \begin{minipage}{0.42\textwidth}
            \centering
            \vskip 40pt
            \includegraphics[width=\linewidth]{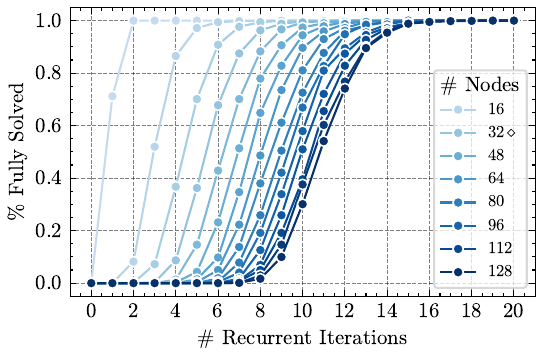}
            \captionof{figure}{Robust out-of-distribution generalization via input-adaptive scaling of computation time. This depicts \methodcolorhighlight{discretesupervisionrecorrectioncolor}{Discrete Latent Space Supervision $\circlearrowleft$}}
            \label{fig:ourmethod_stepwise_results}
    \end{minipage}
\end{figure}

\subsection{Experimental Results \& Discussion}

Combining these mechanisms yields an architecture capable of robustly generalizing far beyond the training distribution to much larger inputs. To evaluate the effects of the different mechanisms we propose, we study a collection of methods implementing different subsets of the mechanisms. This is described in~\Cref{tab:method_guide}.

\textbf{\textit{A Dramatic Improvement in Out-of-Distribution Generalization.}} \Cref{fig:method_ood_comparison} depicts the out-of-distribution generalization performance of several versions of our method, ablating across the ingredients described above, as well as the aforementioned \methodcolorhighlight{cotsupervisioncolor}{Chain-of-Thought} and \methodcolorhighlight{feedforwardcolor}{End-to-End} baselines. As previously mentioned, we find that the end-to-end models fail to robustly learn the task (with respect to our stringent ``fully solved'' metric) beyond small graph sizes, even in-distribution. The recurrent models slightly outperform the feedforward models. Chain-of-Thought supervision enables a significant improvement, yielding near-perfect performance in-distribution, and a limited degree of out-of-distribution generalization. To assess our proposed mechanisms for robust OOD generalization in Transformers, we evaluate three classes of models incorporating different subsets of those ingredients. We find that this enables a dramatic improvement in OOD generalization, with further improvement the more ingredients are incorporated. When all proposed ingredients are incorporated, the model robustly achieves near-perfect performance across all OOD splits we examined.

\textbf{\textit{The Importance of Anchored Discrete Representations.}} In~\Cref{fig:method_ood_comparison}, \methodcolorhighlight{continuoussupervisioncolor}{Continuous Latent Space Supervision} denotes a recurrent model where the continuous latent states receive step-by-step algorithmic supervision, but the latent states are not discretized in between recurrent block iterations as they are in \methodcolorhighlight{discretesupervisioncolor}{Discrete Latent Space Supervision}. We see that, while this outperforms the chain-of-thought baseline which is limited to linear reasoning paths, its out-of-distribution performance slowly degrades as we test on progressively larger inputs which require increasing recurrent depth and computation time. We attribute this to accumulating noise in the continuous vector representations as we scale test-time compute in order to solve larger problem instances that eventually cause representations to drift from the semantically meaningful manifold learned during training. In \methodcolorhighlight{discretesupervisioncolor}{Discrete Latent Space Supervision}, the model receives step-by-step algorithmic supervision as with its continuous counterpart, but now we additionally discretize the latent representation, then re-embed using a common embedder that is shared across recurrent iterations. This has the effect of ``pinning'' the latent states to a common, semantically-consistent representation space, allowing the model to scale up computational depth without accumulating noise. We observe that this yields significantly improved OOD generalization.
\aanote{Can this be related, intuitively, to ideas from coding theory? Channel coding, etc.}
\aanote{This resembles the method explored in~\citet{dengImplicitChainThought2023,dengExplicitCoTImplicit2024}, where the continuous hidden states of the model are utilized for reasoning. {TODO--Look at this work in more detail, and see if there is any other relevant work to cite here. Include in discussion/related work.}}

\textbf{\textit{Error-Correction Leads to Greater Robustness in Scaling.}} 
% In our initial experiments, we found that, even without explicitly training the model to correct its errors, the \methodcolorhighlight{discretesupervisioncolor}{Discrete Latent Space Supervision} model is able to correct errors from the previous iteration about 50\% of the time per step. 
In \methodcolorhighlight{discretesupervisionrecorrectioncolor}{Discrete Latent Space Supervision $\circlearrowleft$}, we introduce explicit supervision for error correction by randomly corrupting the model's latent space with some small probability during training. 
While the resulting model occasionally makes errors, it is able to correct its errors in the next recurrent iteration nearly 100\% of the time, in turn yielding robust near-perfect OOD generalization.
% This boosts the 1-step error correction probability to nearly 100\% and in turn enables robust near-perfect OOD generalization across all OOD splits. 
Interestingly, we find that error correction requires more layers in the recurrent block in order to succeed. This is intuitive, since it requires additional computational depth from the model per-step to first detect and correct errors from previous steps, before performing the computation for the current step.

\textbf{\textit{Robust Test-time Scaling.}} On many tasks, the computation time required to solve a problem instance is proportional to its size or complexity. Consequently, solving problems larger than those encountered during training necessitates scaling computation time beyond the training regime. In our setting, where the model's reasoning process is latent, we achieve this by increasing the number of recurrent iterations. \Cref{fig:ourmethod_stepwise_results} depicts the proportion of input instances solved as a function of the number of recurrent iterations. Increasing the number of iterations enables solving incrementally larger and harder problem instances. Our architectural mechanisms enable this robust scaling beyond the training regime.

\aanote{Contrast this with prior work on test-time scaling, where it is found that there are hard limits and performance plateaus. E.g.,~\citet{geipingScalingTestTimeCompute2025}: does not really scale beyond the training regime. I.e., scaling compute inside the training range improves performance, but increasing the number of iterations beyond the training regime does not yield improved performance.}

\textbf{\textit{Details, Extensions \& Further Ablations.}} In~\Cref{sec:cot_details,sec:latent_supervision_details,sec:experiments_additional_operations} we provide further discussion and present additional experimental results. Here, we briefly highlight a few aspects of these extensions. Across all methods, we find that hyperparameter choice can be critical. In particular, we find that the choice of positional encoding and model depth is especially important. In the above results, we always report the best model with each method after a hyperparameter search, the details of which are provided in the appendix. Additionally, for the chain-of-thought baselines, we explore multiple schemes for the design of the reasoning chains and present the best results here. We also discuss applying our method to more challenging task setups with multiple arithmetic operations.

% Here, we will focus on a version of the task with a single operation, modular addition, since our focus is on studying out-of-distribution generalization, and traditional methods such as linear chain-of-thought training fail even in this simpler setting. In~\Cref{sec:experiments_additional_operations} we apply our method to a more complex setting with several operations, where the model must learn several operations.

Now that we've demonstrated the effectiveness of the proposed architectural mechanisms for robust OOD generalization, we next conduct a mechanistic interpretability analysis to probe the precise computational circuits learned by each component of our model.
