# Supplementary material for: Unlocking Out-of-Distribution Generalization in Transformers via Recursive Latent Space Reasoning
Source: arXiv:2510.14095 source file (2025-10-15)
Supplement: Supplementary file 3 [file all_models_fullseqacc_table.tex]

\begin{tabular}{lr}
\toprule
Model & Full Sequence Accuracy \\
\midrule
SinAbPE-T1L2H16D256 & 0.4\% \\
SinAbPE-T1L2H16D512 & 0.9\% \\
SinAbPE-T1L8H16D256 & 14.7\% \\
SinAbPE-T2L2H16D256 & 8.9\% \\
SinAbPE-T2L2H16D512 & 13.2\% \\
SinAbPE-T2L4H16D256 & 14.5\% \\
SinAbPE-T4L2H16D256 & 14.4\% \\
AbPE-T1L2H16D256 & 2.7\% \\
AbPE-T1L2H16D512 & 2.8\% \\
AbPE-T2L2H16D256 & 11.5\% \\
AbPE-T2L2H16D512 & 10.4\% \\
AbPE-T4L2H16D256 & 13.2\% \\
AbPE-T4L2H16D512 & 0.0\% \\
RoPE-T1L2H16D256 & 1.8\% \\
RoPE-T1L2H16D512 & 1.0\% \\
RoPE-T1L8H16D256 & 12.2\% \\
RoPE-T2L2H16D256 & 9.8\% \\
RoPE-T2L2H16D512 & 10.8\% \\
RoPE-T4L2H16D256 & 16.2\% \\
RoPE-T4L2H16D512 & 0.0\% \\
NoPE-T1L2H16D256 & 0.1\% \\
NoPE-T1L2H16D512 & 0.2\% \\
NoPE-T1L8H16D256 & 12.7\% \\
NoPE-T2L2H16D256 & 5.2\% \\
NoPE-T2L2H16D512 & 7.6\% \\
NoPE-T2L4H16D256 & 11.8\% \\
NoPE-T4L2H16D256 & 10.2\% \\
NoPE-T4L2H16D512 & 0.0\% \\
DeBERTa-T1L2H16D256 & 1.9\% \\
DeBERTa-T1L2H16D512 & 1.1\% \\
DeBERTa-T1L8H16D256 & 15.0\% \\
DeBERTa-T2L2H16D256 & 2.6\% \\
DeBERTa-T2L2H16D512 & 6.4\% \\
DeBERTa-T2L4H16D256 & 15.0\% \\
DeBERTa-T4L2H16D256 & 14.7\% \\
DeBERTa-T4L2H16D512 & 8.5\% \\
\bottomrule
\end{tabular}
