# Supplementary material for: Unlocking Out-of-Distribution Generalization in Transformers via Recursive Latent Space Reasoning
Source: arXiv:2510.14095 source file (2025-10-15)
Supplement: Supplementary file 5 [file all_models_fullseqacc_table.tex]

\begin{tabular}{lllr}
\toprule
PosEnc & CoT Type & Architecture & All Sequence Accuracy \\
\midrule
RoPE & Eq-Val & T1L4H16D256 & 5.2\% \\
RoPE & Eq-Val & T1L8H16D256 & 5.3\% \\
RoPE & Eq-Val & T2L4H16D256 & 4.0\% \\
RoPE & Eq-Val & T4L2H16D256 & 0.0\% \\
RoPE & Eq-Val (Var Len) & T1L4H16D256 & 1.8\% \\
RoPE & Eq-Val (Var Len) & T1L8H16D256 & 0.0\% \\
RoPE & Val & T1L4H16D256 & 0.0\% \\
RoPE & Val & T4L2H16D256 & 2.6\% \\
RoPE & Val (Var Len) & T1L4H16D256 & 0.2\% \\
RoPE & Val (Var Len) & T1L8H16D256 & 23.8\% \\
NoPE & Eq-Val (Var Len) & T1L8H16D256 & 33.6\% \\
NoPE & Eq-Val (Var Len) & T1L8H16D512 & 35.4\% \\
NoPE & Val & T1L2H16D256 & 0.0\% \\
NoPE & Val & T1L2H16D512 & 0.0\% \\
NoPE & Val & T2L2H16D256 & 0.0\% \\
NoPE & Val & T2L2H16D512 & 0.4\% \\
NoPE & Val & T4L2H16D256 & 0.0\% \\
NoPE & Val & T4L2H16D512 & 0.0\% \\
DeBERTa & Eq-Val & T1L4H16D256 & 7.0\% \\
DeBERTa & Eq-Val & T1L8H16D256 & 22.4\% \\
DeBERTa & Eq-Val & T4L2H16D256 & 0.0\% \\
DeBERTa & Eq-Val (Var Len) & T1L4H16D256 & 0.1\% \\
DeBERTa & Val & T1L2H16D256 & 0.0\% \\
DeBERTa & Val & T1L2H16D512 & 0.0\% \\
DeBERTa & Val & T1L4H16D256 & 0.0\% \\
DeBERTa & Val & T1L8H16D256 & 0.0\% \\
DeBERTa & Val & T1L8H16D512 & 0.0\% \\
DeBERTa & Val & T2L2H16D256 & 0.0\% \\
DeBERTa & Val & T2L2H16D512 & 0.0\% \\
DeBERTa & Val & T2L4H16D256 & 0.3\% \\
DeBERTa & Val & T2L4H16D512 & 0.0\% \\
DeBERTa & Val & T4L2H16D256 & 0.0\% \\
DeBERTa & Val & T4L2H16D512 & 0.0\% \\
DeBERTa & Val (Var Len) & T1L4H16D256 & 5.0\% \\
DeBERTa & Val (Var Len) & T1L8H16D256 & 23.3\% \\
\bottomrule
\end{tabular}
