# Supplementary material for: Unlocking Out-of-Distribution Generalization in Transformers via Recursive Latent Space Reasoning
Source: arXiv:2510.14095 source file (2025-10-15)
Supplement: Supplementary file 6 [file all_models_tokenwiseacc_table.tex]

\begin{tabular}{lllr}
\toprule
PosEnc & CoT Type & Architecture & All Tokenwise Accuracy \\
\midrule
RoPE & Eq-Val & T1L4H16D256 & 15.2\% \\
RoPE & Eq-Val & T1L8H16D256 & 20.4\% \\
RoPE & Eq-Val & T2L4H16D256 & 14.9\% \\
RoPE & Eq-Val & T4L2H16D256 & 15.8\% \\
RoPE & Eq-Val (Var Len) & T1L4H16D256 & 24.6\% \\
RoPE & Eq-Val (Var Len) & T1L8H16D256 & 16.1\% \\
RoPE & Val & T1L4H16D256 & 19.7\% \\
RoPE & Val & T4L2H16D256 & 24.2\% \\
RoPE & Val (Var Len) & T1L4H16D256 & 37.1\% \\
RoPE & Val (Var Len) & T1L8H16D256 & 42.7\% \\
NoPE & Eq-Val (Var Len) & T1L8H16D256 & 50.2\% \\
NoPE & Eq-Val (Var Len) & T1L8H16D512 & 53.6\% \\
NoPE & Val & T1L2H16D256 & 14.2\% \\
NoPE & Val & T1L2H16D512 & 14.7\% \\
NoPE & Val & T2L2H16D256 & 14.8\% \\
NoPE & Val & T2L2H16D512 & 20.3\% \\
NoPE & Val & T4L2H16D256 & 18.2\% \\
NoPE & Val & T4L2H16D512 & 18.6\% \\
DeBERTa & Eq-Val & T1L4H16D256 & 46.3\% \\
DeBERTa & Eq-Val & T1L8H16D256 & 58.6\% \\
DeBERTa & Eq-Val & T4L2H16D256 & 14.7\% \\
DeBERTa & Eq-Val (Var Len) & T1L4H16D256 & 37.4\% \\
DeBERTa & Val & T1L2H16D256 & 30.9\% \\
DeBERTa & Val & T1L2H16D512 & 32.0\% \\
DeBERTa & Val & T1L4H16D256 & 39.4\% \\
DeBERTa & Val & T1L8H16D256 & 39.0\% \\
DeBERTa & Val & T1L8H16D512 & 37.3\% \\
DeBERTa & Val & T2L2H16D256 & 31.2\% \\
DeBERTa & Val & T2L2H16D512 & 33.4\% \\
DeBERTa & Val & T2L4H16D256 & 23.2\% \\
DeBERTa & Val & T2L4H16D512 & 30.4\% \\
DeBERTa & Val & T4L2H16D256 & 36.0\% \\
DeBERTa & Val & T4L2H16D512 & 0.0\% \\
DeBERTa & Val (Var Len) & T1L4H16D256 & 57.8\% \\
DeBERTa & Val (Var Len) & T1L8H16D256 & 69.5\% \\
\bottomrule
\end{tabular}
