# Supplementary material for: Unlocking Out-of-Distribution Generalization in Transformers via Recursive Latent Space Reasoning
Source: arXiv:2510.14095 source file (2025-10-15)
Supplement: Supplementary file 7 [file all_models_valuetokenwiseacc_table.tex]

\begin{tabular}{lllr}
\toprule
PosEnc & CoT Type & Architecture & Value Tokenwise Accuracy \\
\midrule
RoPE & Eq-Val & T1L4H16D256 & 10.3\% \\
RoPE & Eq-Val & T1L8H16D256 & 14.4\% \\
RoPE & Eq-Val & T2L4H16D256 & 12.2\% \\
RoPE & Eq-Val & T4L2H16D256 & 4.6\% \\
RoPE & Eq-Val (Var Len) & T1L4H16D256 & 18.2\% \\
RoPE & Eq-Val (Var Len) & T1L8H16D256 & 13.8\% \\
RoPE & Val & T1L4H16D256 & 6.9\% \\
RoPE & Val & T4L2H16D256 & 12.1\% \\
RoPE & Val (Var Len) & T1L4H16D256 & 16.0\% \\
RoPE & Val (Var Len) & T1L8H16D256 & 32.4\% \\
NoPE & Eq-Val (Var Len) & T1L8H16D256 & 42.9\% \\
NoPE & Eq-Val (Var Len) & T1L8H16D512 & 44.1\% \\
NoPE & Val & T1L2H16D256 & 4.9\% \\
NoPE & Val & T1L2H16D512 & 7.7\% \\
NoPE & Val & T2L2H16D256 & 6.6\% \\
NoPE & Val & T2L2H16D512 & 7.8\% \\
NoPE & Val & T4L2H16D256 & 5.9\% \\
NoPE & Val & T4L2H16D512 & 4.9\% \\
DeBERTa & Eq-Val & T1L4H16D256 & 40.1\% \\
DeBERTa & Eq-Val & T1L8H16D256 & 92.2\% \\
DeBERTa & Eq-Val & T4L2H16D256 & 7.5\% \\
DeBERTa & Eq-Val (Var Len) & T1L4H16D256 & 22.2\% \\
DeBERTa & Val & T1L2H16D256 & 22.6\% \\
DeBERTa & Val & T1L2H16D512 & 18.5\% \\
DeBERTa & Val & T1L4H16D256 & 19.4\% \\
DeBERTa & Val & T1L8H16D256 & 23.8\% \\
DeBERTa & Val & T1L8H16D512 & 28.4\% \\
DeBERTa & Val & T2L2H16D256 & 10.1\% \\
DeBERTa & Val & T2L2H16D512 & 8.7\% \\
DeBERTa & Val & T2L4H16D256 & 13.6\% \\
DeBERTa & Val & T2L4H16D512 & 14.1\% \\
DeBERTa & Val & T4L2H16D256 & 28.9\% \\
DeBERTa & Val & T4L2H16D512 & NaN \\
DeBERTa & Val (Var Len) & T1L4H16D256 & 31.1\% \\
DeBERTa & Val (Var Len) & T1L8H16D256 & 72.7\% \\
\bottomrule
\end{tabular}
