# Supplementary material for: Unlocking Out-of-Distribution Generalization in Transformers via Recursive Latent Space Reasoning
Source: arXiv:2510.14095 source file (2025-10-15)
Supplement: Supplementary file 8 [file all_models_varfullseqacc_table.tex]

\begin{tabular}{lllr}
\toprule
PosEnc & CoT Type & Architecture & Var Sequence Accuracy \\
\midrule
RoPE & Eq-Val & T1L4H16D256 & 6.2\% \\
RoPE & Eq-Val & T1L8H16D256 & 7.2\% \\
RoPE & Eq-Val & T2L4H16D256 & 8.4\% \\
RoPE & Eq-Val & T4L2H16D256 & 3.0\% \\
RoPE & Eq-Val (Var Len) & T1L4H16D256 & 12.5\% \\
RoPE & Eq-Val (Var Len) & T1L8H16D256 & 1.2\% \\
RoPE & Val & T1L4H16D256 & 44.9\% \\
RoPE & Val & T4L2H16D256 & 6.7\% \\
RoPE & Val (Var Len) & T1L4H16D256 & 24.9\% \\
RoPE & Val (Var Len) & T1L8H16D256 & 25.0\% \\
NoPE & Eq-Val (Var Len) & T1L8H16D256 & 35.4\% \\
NoPE & Eq-Val (Var Len) & T1L8H16D512 & 37.2\% \\
NoPE & Val & T1L2H16D256 & 15.4\% \\
NoPE & Val & T1L2H16D512 & 43.2\% \\
NoPE & Val & T2L2H16D256 & 8.9\% \\
NoPE & Val & T2L2H16D512 & 11.9\% \\
NoPE & Val & T4L2H16D256 & 26.6\% \\
NoPE & Val & T4L2H16D512 & 35.2\% \\
DeBERTa & Eq-Val & T1L4H16D256 & 29.1\% \\
DeBERTa & Eq-Val & T1L8H16D256 & 57.1\% \\
DeBERTa & Eq-Val & T4L2H16D256 & 5.4\% \\
DeBERTa & Eq-Val (Var Len) & T1L4H16D256 & 14.5\% \\
DeBERTa & Val & T1L2H16D256 & 57.7\% \\
DeBERTa & Val & T1L2H16D512 & 11.3\% \\
DeBERTa & Val & T1L4H16D256 & 8.5\% \\
DeBERTa & Val & T1L8H16D256 & 60.8\% \\
DeBERTa & Val & T1L8H16D512 & 2.9\% \\
DeBERTa & Val & T2L2H16D256 & 16.0\% \\
DeBERTa & Val & T2L2H16D512 & 27.4\% \\
DeBERTa & Val & T2L4H16D256 & 55.7\% \\
DeBERTa & Val & T2L4H16D512 & 0.0\% \\
DeBERTa & Val & T4L2H16D256 & 7.1\% \\
DeBERTa & Val & T4L2H16D512 & 100.0\% \\
DeBERTa & Val (Var Len) & T1L4H16D256 & 28.7\% \\
DeBERTa & Val (Var Len) & T1L8H16D256 & 87.9\% \\
\bottomrule
\end{tabular}
