# Supplementary material for: Unlocking Out-of-Distribution Generalization in Transformers via Recursive Latent Space Reasoning
Source: arXiv:2510.14095 source file (2025-10-15)
Supplement: Supplementary file 11 [file best_valuetokenwisacc_by_posenc_table.tex]

\begin{tabular}{lr}
\toprule
PosEnc & Value Tokenwise Accuracy \\
\midrule
SinAbPE & NaN \\
AbPE & NaN \\
RoPE & 32.4\% \\
NoPE & 44.1\% \\
DeBERTa & 72.7\% \\
\bottomrule
\end{tabular}
