# Supplementary material for: Unlocking Out-of-Distribution Generalization in Transformers via Recursive Latent Space Reasoning
Source: arXiv:2510.14095 source file (2025-10-15)
Supplement: Supplementary file 12 [file all_models_fullseqacc_table.tex]

\begin{tabular}{lr}
\toprule
Model & Full Sequence Accuracy \\
\midrule
AbPE - L2H16D256 & 6.2\% \\
AbPE - L4H16D256 & 21.9\% \\
RoPE - L2H16D256 & 16.2\% \\
RoPE - L4H16D256 & 33.7\% \\
NoPE - L2H16D256 & 17.5\% \\
DeBERTa - L2H16D256 & 78.6\% \\
DeBERTa - L2H16D512 & 7.2\% \\
DeBERTa - L4H16D256 & 18.9\% \\
\bottomrule
\end{tabular}
