# Supplementary material for: Unlocking Out-of-Distribution Generalization in Transformers via Recursive Latent Space Reasoning
Source: arXiv:2510.14095 source file (2025-10-15)
Supplement: Supplementary file 13 [file best_fullseqacc_by_architecture_table.tex]

\begin{tabular}{lr}
\toprule
Architecture & Full Sequence Accuracy \\
\midrule
 L2H16D256 & 78.6\% \\
 L2H16D512 & 7.2\% \\
 L4H16D256 & 33.7\% \\
\bottomrule
\end{tabular}
