# Supplementary material for: Unlocking Out-of-Distribution Generalization in Transformers via Recursive Latent Space Reasoning
Source: arXiv:2510.14095 source file (2025-10-15)
Supplement: Supplementary file 15 [file best_fullseqacc_by_architecture_table.tex]

\begin{tabular}{lr}
\toprule
Architecture & Full Sequence Accuracy \\
\midrule
 L2H16D256 & 96.5\% \\
 L2H16D512 & 89.0\% \\
 L4H16D256 & 86.5\% \\
 L4H16D384 & 97.8\% \\
\bottomrule
\end{tabular}
