# Supplementary material for: Unlocking Out-of-Distribution Generalization in Transformers via Recursive Latent Space Reasoning
Source: arXiv:2510.14095 source file (2025-10-15)
Supplement: Supplementary file 16 [file best_fullseqacc_by_posenc_table.tex]

\begin{tabular}{lr}
\toprule
PosEnc & Full Sequence Accuracy \\
\midrule
SinAbPE & NaN \\
AbPE & 19.9\% \\
RoPE & 30.5\% \\
NoPE & 30.4\% \\
DeBERTa & 97.8\% \\
\bottomrule
\end{tabular}
